# Supplementary material for: Tagvisor: A Privacy Advisor for Sharing Hashtags
Source: arXiv:1802.04122 source file (2018-02-12)
Supplement: Supplementary file 1 [file appendix.tex]

\section{Additional Figures}
\label{sec:additional_evalua}
%Figure~\ref{figure:cnt_accuracy} depicts the average accuracy for the two adversary models with different number of hashtags in a photo.
\begin{figure*}
\centering
\subfigure[]{
\includegraphics[width=0.9\columnwidth]{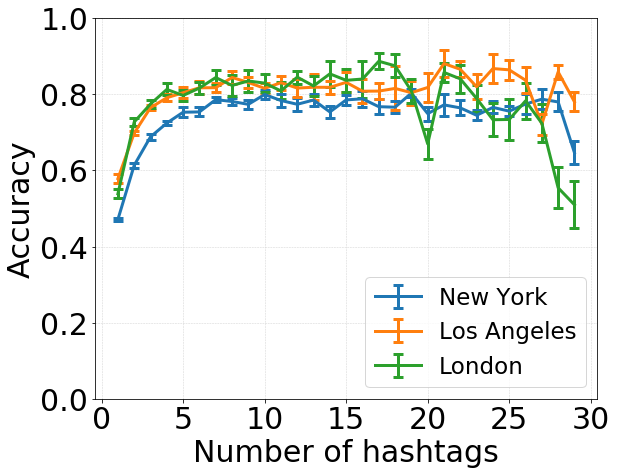}}
\subfigure[]{
\includegraphics[width=0.9\columnwidth]{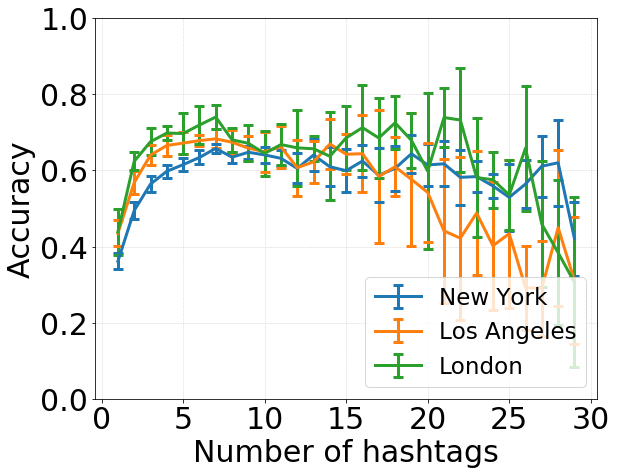}}
\caption{Accuracy of adversary (a) $\Adversary_1$ and 
(b) $\Adversary_2$
for posts with different number of hashtags.}
\end{figure*}

\begin{figure*}
	\centering
	\subfigure[]{\includegraphics[width=0.68\columnwidth]{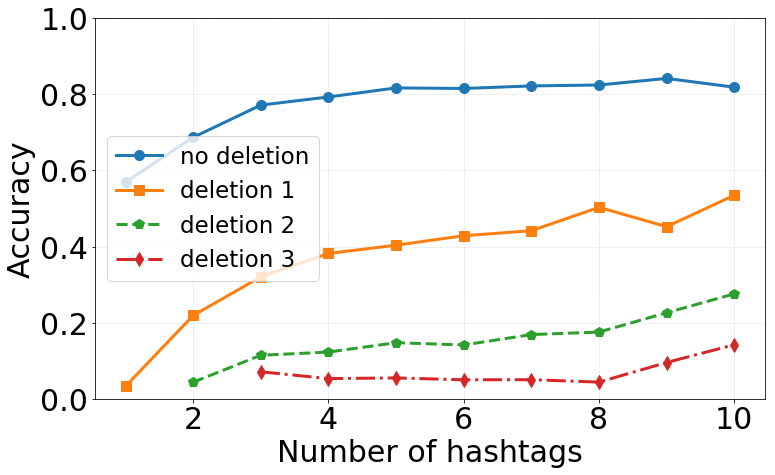}}
    \subfigure[]{\includegraphics[width=0.68\columnwidth]{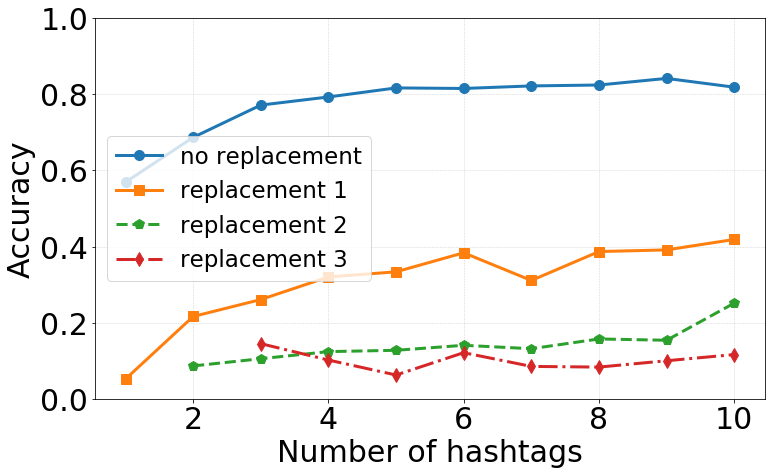}}
    \subfigure[]{\includegraphics[width=0.68\columnwidth]{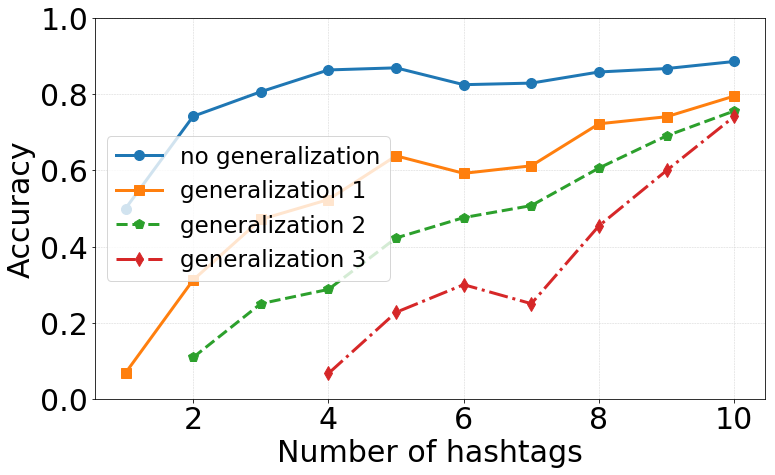}}
    \caption{Evolution of the accuracy ($\Adversary_1$) with respect to different numbers of hashtags to be shared and numbers of obfuscated hashtags for (a) hiding, (b) replacement, and (c) generalization in Los Angeles.}
\end{figure*}

\begin{figure*}
	\centering
	\subfigure[]{\includegraphics[width=0.68\columnwidth]{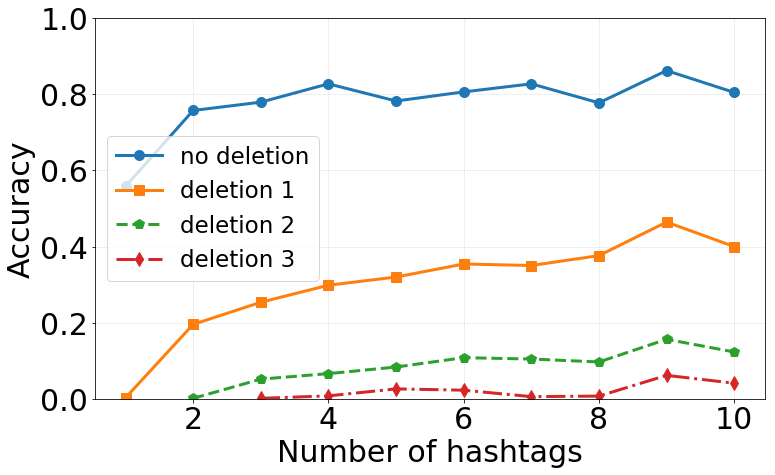}}
    \subfigure[]{\includegraphics[width=0.68\columnwidth]{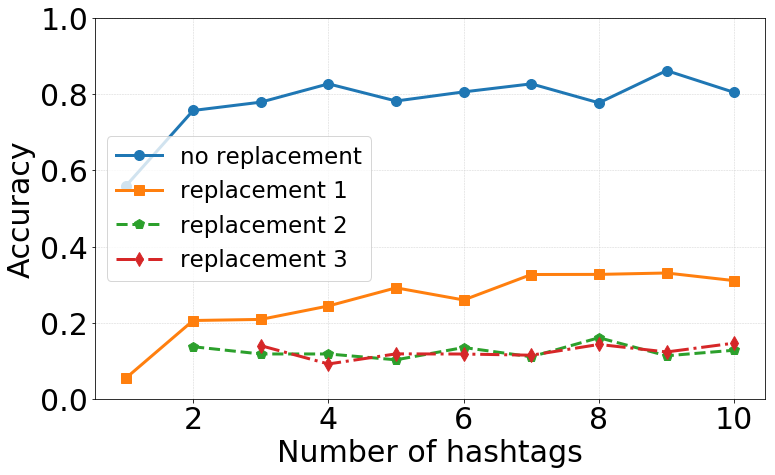}}
    \subfigure[]{\includegraphics[width=0.68\columnwidth]{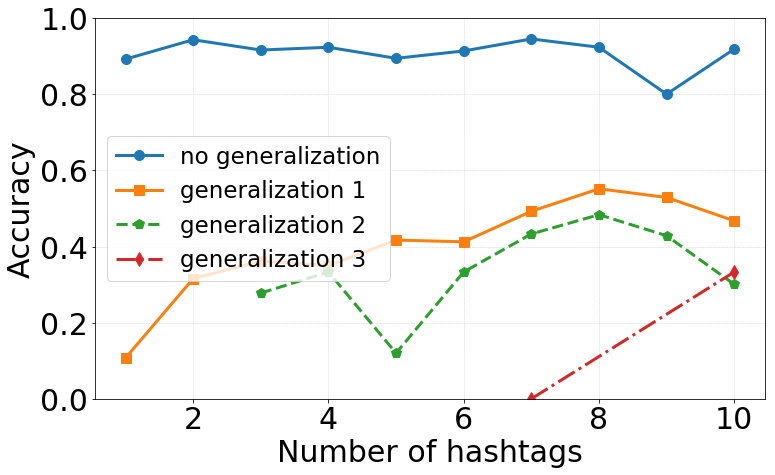}}
    \caption{Evolution of the accuracy ($\Adversary_1$) with respect to different numbers of hashtags to be shared and numbers of obfuscated hashtags for (a) hiding, (b) replacement, and (c) generalization in London.}
\end{figure*}
